# Supplementary material for: Photonic chip-based resonant supercontinuum
Source: arXiv:1909.00022 ancillary file (2020-03-23)
Supplement: Supplementary file 1 [file ResonantSCG_SI_v1.pdf]

# Supplementary Information to Photonic chip-based resonant supercontinuum

Miles H. Anderson,[1] Romain Bouchand,[1] Junqiu Liu,[1] Wenle Weng,[1]
Ewelina Obrzud,[2] Tobias Herr,[2] and Tobias J. Kippenberg[1,*]

[1]*École Polytechnique Fédérale de Lausanne (EPFL), CH-1015 Lausanne, Switzerland*

[2]*Swiss Center for Electronics and Microtechnology (CSEM), Time and frequency, CH-2002 Neuchâtel, Switzerland*

## I. PULSE FORMATION FROM ELECTRO-OPTIC COMB.

Fig. S.1 shows modeling of our EO-comb waveform as it travels through a length of dispersion compensation. The white-dashed line in Fig. S.1(c,d) marks the waveform after 300 m of SMF-28 (6.6 $ps^2$), near its maximum compression to 1.2 ps in width (full-width half-maximum). However, successful formation of dissipative Kerr solitons (DKS) through scanning over resonance was experimentally difficult with this configuration, with long soliton 'steps'[1] failing to appear. Modeling predicts that the phase curvature on the pulse at this point would be either zero or positive (Fig. S.1(d)), which would create an overall phase-based repulsion effect of DKS existing on the pulse[2], in addition to the already present intensity based repulsion from the pulse center towards the edges of the pulse[3]. By adding 5 m of dispersion-compensating fiber (DCF), amounting to $\sim 0.7$ $ps^2$, indicated by the red-dashed line in Fig. S.1(c,d), we bring the pulse back to a point where it is slightly longer at 1.4 ps, and has a negative phase curvature. With this configuration in experiment, we found DKS generation to be more successful with longer steps observed.

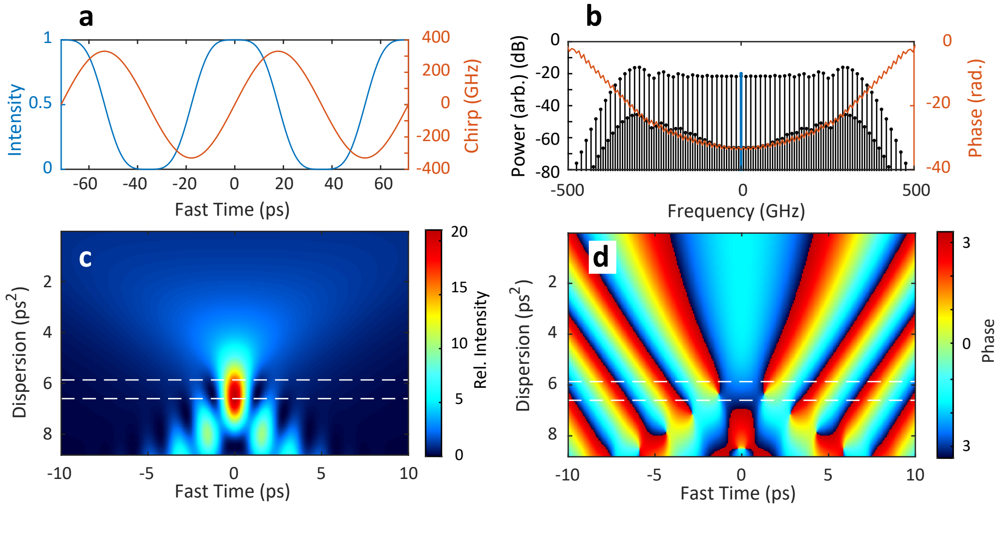


FIG. S.1. **Numerical analysis of EO-comb pulse compression.** (a) Time-domain and (b) spectrum of chirped waveform created from phase-modulation with a depth of $15V_\pi$, and intensity-modulation. (c) Relative EO-comb waveform intensity, and (d) phase vs. propagation through dispersion compensation. Dashed lines mark pulse after 300 m of SMF-28 (6.6 $ps^2$) (white), and 300 m SMF-28 + 5 m DCF (5.9 $ps^2$).

## II. SUPPLEMENTARY MICRORESONATOR AND EXPERIMENTAL DETAILS.

Measurements of the microresonator properties using frequency-comb assisted swept-laser spectroscopy[4] are presented in Fig. S.2. In figure Fig. S.2(b), the cavity modal dispersion $D_{\mathrm{int}}(\mu) = \omega_\mu - \omega_0 - \mu D_1$ is plotted. Fitting to a quadratic $D_{\mathrm{int}} \approx \frac{\mu^2}{2} D_2$ yields $D_2 = 2\pi \cdot 7.2$ kHz ($\beta_2 = -11$ fs$^2$/mm). While the residual deviations from this fit seem apparently significant, this is because of the comparative flatness of the dispersion profile. For comparison, recently posted $Si_3N_4$ microresonators for microwave synthesis have a measured $\beta_2 = -190$ fs$^2$/mm[5]. The distribution of loaded cavity linewidths (close to critical coupling) is plotted in Fig. S.2(c). The peak corresponding to the most probable linewidth is at $\kappa = 2\pi \cdot 110$ MHz, or quality-factor $Q_L = 1.75 \times 10^6$.

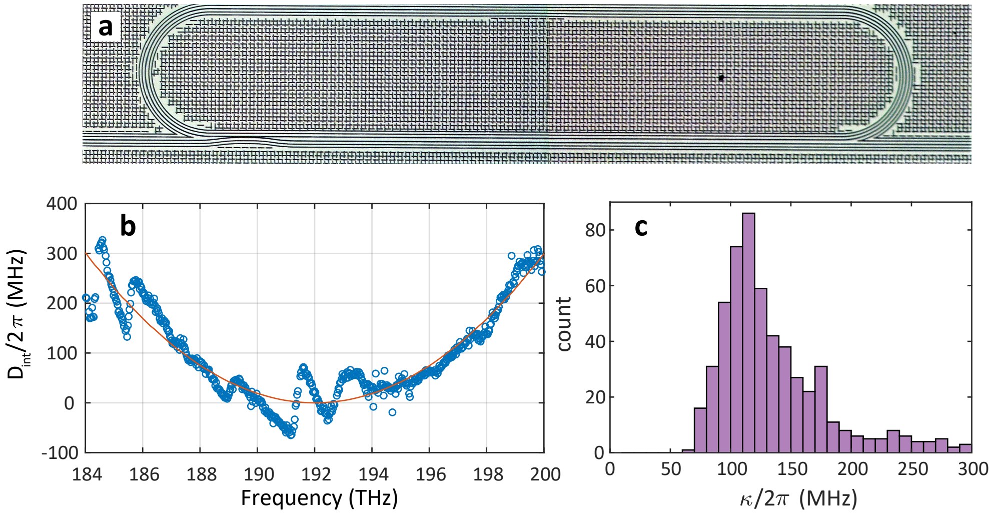


FIG. S.2. **Microresonator properties.** (a) Image of the whole microresonator. (b) Integrated dispersion $D_{\mathrm{int}}$ measurement of 28 GHz mode spectrum (blue), and quadratic fit (red). (c) Histogram of measurements of loaded cavity linewidth $\kappa$.

Fig. S.3(a) shows examples of the power traces measured at the output of the $Si_3N_4$ chip while the laser center frequency is scanned over the cavity resonance, from the blue-detuned to the red-detuned side. Three power levels are shown. The soliton step first appears at 12 mW average coupled to the resonator (41 mW total towards the resonator accounting for insertion loss and sub-harmonic driving). At a mid-range power of 24 mW, DKS tend to form in numbers from 1-3. As shown in the bottom high-power trace at 180 mW, only a single-state is accessible and the step has become substantially longer, enabling easy access to the DKS state using slow tuning of the laser frequency. Example spectra of the DKS multi-states able to formed at a fixed medium power level are shown in Fig. S.3(b).

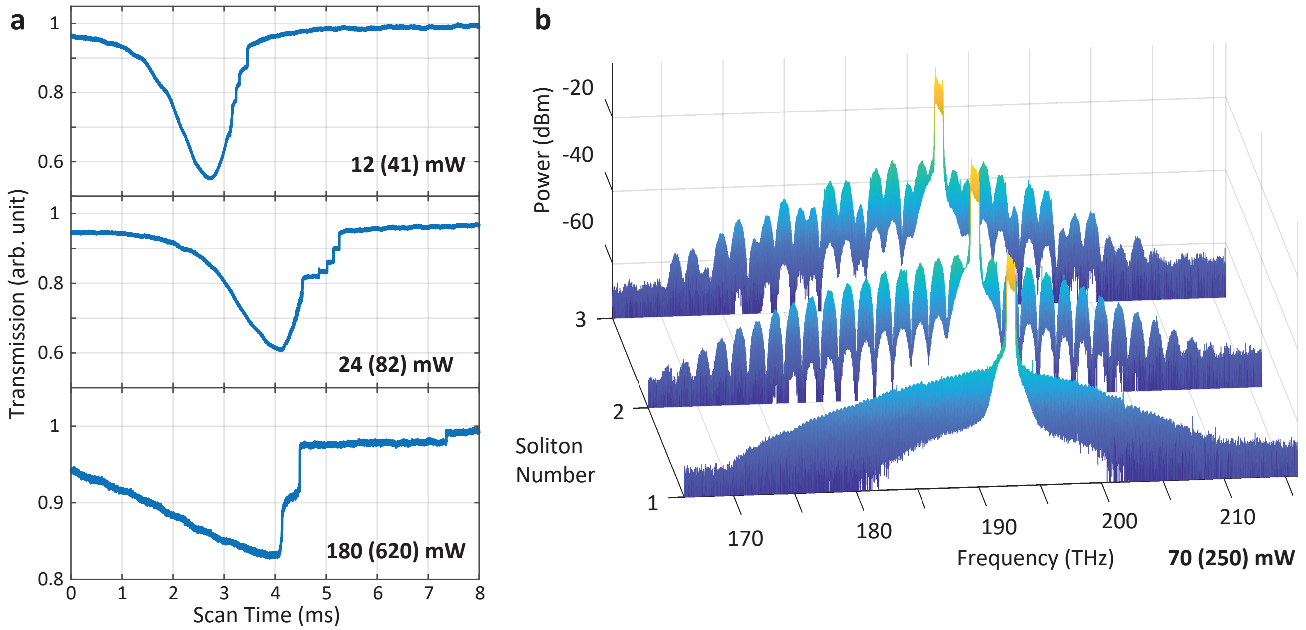


FIG. S.3. **Dissipative Kerr soliton generation and multi-states.** (a) Examples of transmission traces detected at the output of the resonator while the laser is tuned over resonance (in the negative frequency direction), for different input power levels. (b) Example of multi-soliton spectra.

## III. SPECTRAL COHERENCE COMPARED WITH CONVENTIONAL SCG

A question to be answered is how the linewidth of the DKS spectrum, which is subject to nonlinear filtering with bandwidth on the order 1 MHz (see main text), compares to the comb lines of a conventional supercontinuum which has no filtering. In order to measure this, we form a supercontinuum from an EO-comb driven with the same RF sources as in the DKS generation experiment: RF-1 (Rhode & Schwarz SMB100A), and RF-2 (Keysight E8267D). See Fig. 1 of the main text for the frequency noise spectra of these sources. The supercontinuum is formed through a combination of amplification through an EFDA and nonlinear pulse compression in lengths of normal and anomalous dispersion fiber, before creating a supercontinuum through highly-nonlinear fiber. Further details are given in *Obrzud et al.*[6].

The supercontinuum generated from the EO-comb driven by the ultra-low phase-noise signal generator RF-2 is shown in Fig. S.4(a), and the heterodyne beatnote detected at 1908 nm with the same external laser is plotted in Fig. S.4(b) in comparison to the beatnote measured of the same comb tooth from the DKS spectrum. The SCG-based beatnote has a linewidth of $\sim$1.8 MHz, approximately double that of the DKS. When switching RF sources to the higher phase-noise RF-1, it must be reported that the beatnote at 1908 nm was *undetectable* by our experimental means, indicating it was too broad to be resolved with the given equipment due to the noise multiplication. This suggests that it was the DKS-based nonlinear filtering that allowed the DKS-comb beatnote at 1908 nm to be detectable when using RF-1 as the EO-comb modulation source (Fig. 2, 4, in the main text).

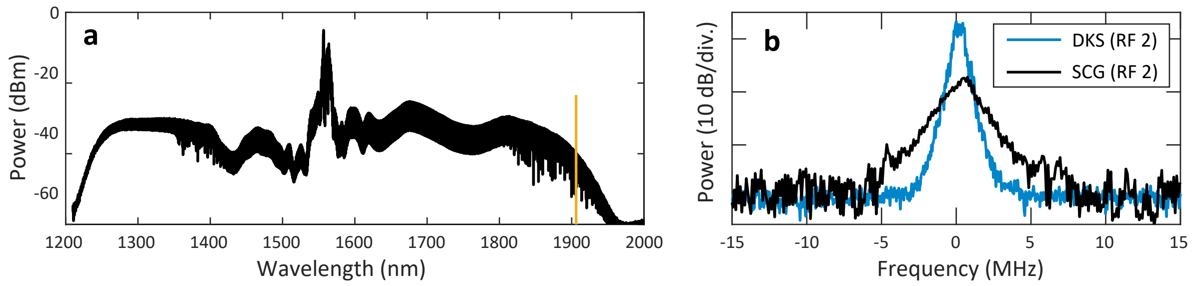


FIG. S.4. (a) EO-comb based supercontinuum spectrum at 14 GHz spacing, with beatnote measurement location marked in yellow. (b) Heterodyne beatnote at 1908 nm measured against the DKS- and supercontinuum-based frequency comb, driven by source RF-2 (RBW = 50 kHz, and 1 MHz respectively).

## IV. DISSIPATIVE SOLITON SIMULATIONS WITH GENERALIZED MEAN-FIELD MODEL

We can model the full spectrum of the generated DKS state (resonant supercontinuum) using the generalized Lugiato-Lefever equation[7,8] (GLLE), including third-order dispersion, the Raman shock[9], and a spectrally variant resonator coupling $\kappa_{\mathrm{ex}}(\mu)$, in the domain of the microresonator longitudinal modes relative to the center wavelength ($\mu = (\omega - \omega_0)/D_1$):

$$\frac{\partial \tilde{A}_\mu(t)}{\partial t} = i\left(\frac{D_2}{2}\mu^2 + \frac{D_3}{6}\mu^3 - \delta\omega\right)\tilde{A}_\mu - \frac{\kappa(\mu)}{2}\tilde{A}_\mu + ig\mathcal{F}\big[(1-f_{\mathrm{R}})|A|^2 A + f_{\mathrm{R}}(h_{\mathrm{R}}(\phi)\otimes|A|^2)A\big] + \sqrt{\kappa_{\mathrm{ex}}(\mu)}F_\mu(t) \quad (1)$$

Here we include dispersion up to the third-order, with $D_2 = 2\pi\cdot 7.2$ kHz measured from Fig. S.2(a), and $D_3 = 2\pi\cdot 15$ Hz estimated *a posteriori* from the location of the dispersive wave on the measured DKS spectrum at $\mu_{\mathrm{DW}} = -1400$, where $-3D_2/D_3 = \mu_{\mathrm{DW}}$. The nonlinear coupling term $g = \hbar\omega_0^2 v_g^2 n_2/(cA_{\mathrm{eff}}L)$ describes the resonance frequency shift per photon for a cavity of effective volume $A_{\mathrm{eff}}L$, material nonlinear refractive index $n_2 = 2.4\times 10^{-19}$ m$^2$/W, and waveguide group velocity $v_g = 1.444\times 10^8$ m/s. Using a finite-element method calculation based on the 2.35×0.77 µm$^2$ waveguide cross-section, we obtain an effective mode area of $1.46\times 10^{-12}$ m$^2$ at the center frequency $\omega_0 = 2\pi\cdot 192$ THz. With the resonator length of $5.18\times 10^{-3}$ m, we find $g = 2\pi\cdot 0.054$ Hz. We take the Raman contribution $f_{\mathrm{R}} = 0.2$, and based on prior work[9], we assume a linear approximation of the Raman response such that

$$h_{\mathrm{R}}(\phi)\otimes|A|^2 \approx |A|^2 - \tau_R D_1\frac{\partial|A|^2}{\partial\phi} \quad (2)$$

with Raman 'shock' time $\tau_R = 20$ fs. The cavity dissipation $\kappa = \kappa_0 + \kappa_{\mathrm{ex}}(\omega)$, and the external coupling rate $\kappa_{\mathrm{ex}}(\omega) = \theta(\omega)D_1/2\pi$, where $\theta(\omega)$ is the bus-resonator coupling coefficient. Due to the 30 µm long straight coupling section, $\theta(\omega)$ that has a strong decline with increasing optical frequency, which we model with a simple exponential decay:

$$\theta(\omega) = \frac{1}{1 + e^{\alpha(\omega-\omega_0)}/\theta_0} \quad (3)$$

where $\theta_0$ is the coupling coefficient at the pump wavelength $\omega_0$ ($\theta_0 \ll 1$), and $\alpha$ is the coupling decay constant. Based on measurements of the microresonator, we set $\theta_0 = 0.011$ so that $\kappa_{\mathrm{ex}}(\mu = 0) = 2\pi\cdot 50$ MHz, and $\kappa_0 = 2\pi\cdot 50$ MHz so as to be critically coupled. We choose $\alpha = 7\times 10^9$ /Hz. Finally, the input pulse spectrum $F_\mu$ is defined as

$$F_\mu = \frac{\sqrt{P_0/\hbar\omega_0}}{M+1}\,\Pi\big(\mu/(M+1)\big)e^{i\hat{D}_c} \quad (4)$$

With $\Pi(\mu)$ being the rectangular function, and $M = 24$ being the number of EO-comb lines in addition to the seed pump line, and pulse peak power $P_0$ (at minimum pulse duration). The peak power can be expressed in terms of the threshold for parametric sideband formation[10,11] as $P_0 = f^2 P_{\mathrm{th}}$, where $P_{\mathrm{th}} = \hbar\omega_0\kappa^3/(8\kappa_{\mathrm{ex}}g)$. Additional dispersion

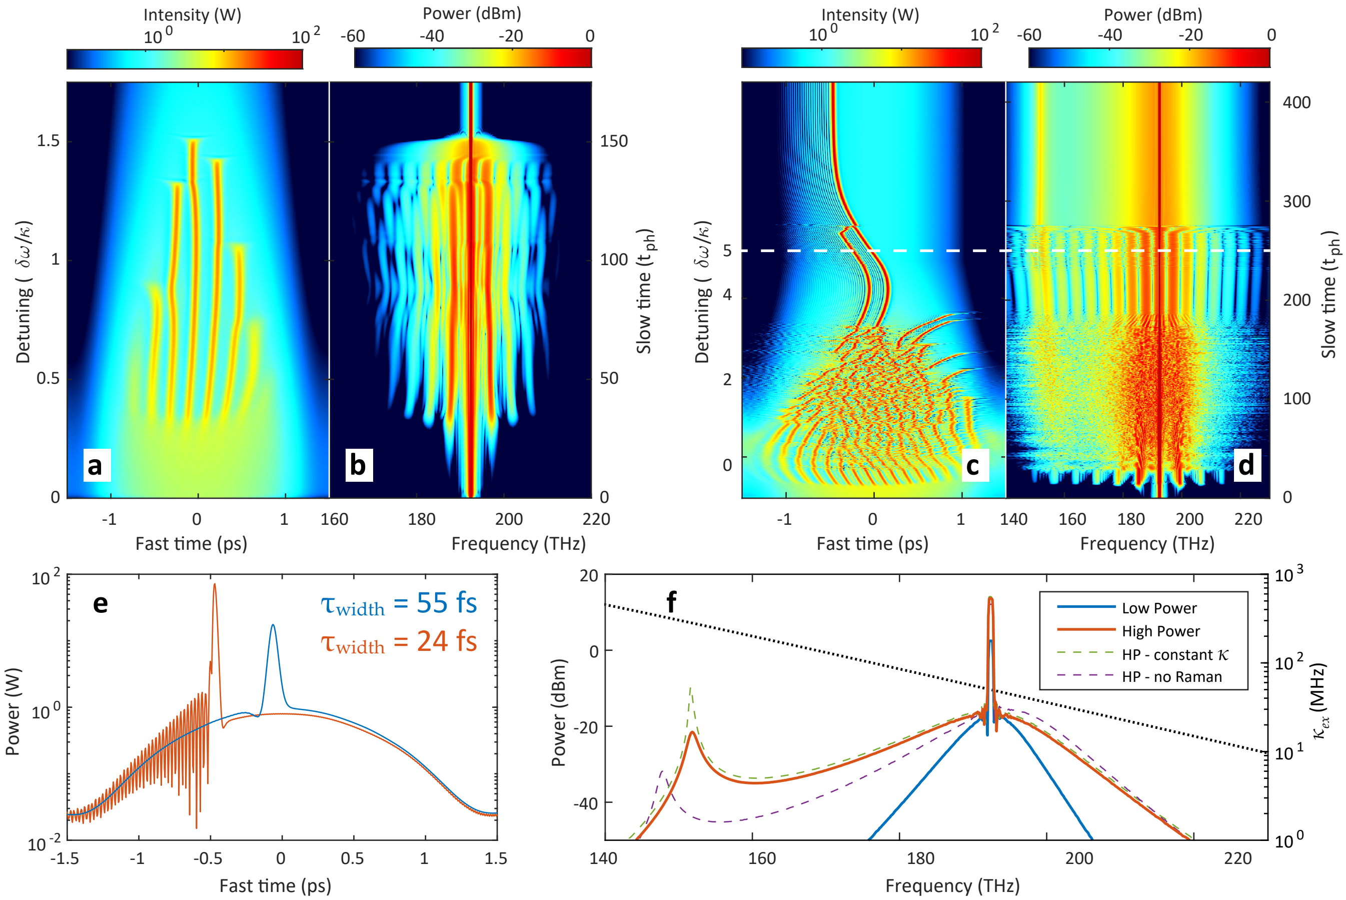


FIG. S.5. **Dissipative Kerr soliton formation simulation based on the generalized Lugiato-Lefever equation.** (a) Intracavity optical field and (b) frequency domain output over change in $\delta\omega$ (scan over resonance), at low power. (b,c) Same as (a,b) for high power. Laser frequency tuning stops at white-dashed line. (e) Intracavity time-domain slices of stable single DKS state for low (blue) and high (red) power and detuning. (f) Final output spectrum for single-DKS states (solid line), and the same high power DKS with perturbations removed (dashed line), and $\kappa_{\mathrm{ex}}(\omega)$ (dotted line).

is applied to the pulse spectrum with the term $e^{i\hat{D}_c}$, where $\hat{D}_c = \beta_c(\mu D_1)^2/2$. We choose an intermediate value of added dispersion $\beta_c = 0.3$ ps$^2$, within the bounds given in Fig. S.1(c).

In Fig. S.5, we present an example simulation re-creating the DKS generation in the experiment, giving some insight into how strongly perturbed solitons form on the input pulse and the roles played by the higher-order terms in the GLLE. In Fig. S.5(a,b) we show how DKS are formed during a scan of the laser frequency over resonance at low power, where $P_0 = 100$ mW or $2.5P_{\mathrm{th}}$. In this scenario, the solitons exist well below the instability thresholds and so do not exhibit any breathing or chaos[12], and they have a small existence range over detuning, as also seen in the corresponding low-power experimental trace shown in Fig. S.3(a). Formed solitons collapse one by one when the local power level beneath each of them drops below its minimum. Stopping the scan before the last soliton collapse leaves the low energy traces (blue) in Fig. S.5(e,f), showing a profile very close to the typical sech$^2$ DKS profile, and matching the character of the experimentally generated low-energy DKS shown in the main text Fig. 2(c).

The formation of a DKS at high power is shown in Fig. S.5(c,d), where $P_0 = 25P_{\mathrm{th}}$. At this driving strength, stable Turing rolls[13] form at a low detuning ($\delta\omega < 0$), before entering into a regime of turbulence[14] up until $\delta\omega < 3\kappa$. At this point solitons form in the region of bistability, featuring strong dispersive wave tails (soliton Cherenkov radiation[15]). For the rest of scan until $\delta\omega = 5\kappa$, the group velocity of the soliton curves due to the competing shifts in the spectral center from the counter-acting effects of dispersive-wave induced recoil[16], and the Raman self-frequency shift[9]. By the end, the dispersive-wave recoil becomes dominant. For this simulated example, the whole pulse-background has a repetition-rate mismatch (ie. group velocity shift) of $d = -50$ kHz so as to contain the shifting solitons inside their locking range with the pulse.

The scan is stopped at $\delta\omega = 5\kappa$ leaving a bound dual-soliton state moving towards the pulse edge. As has also been shown in recent numerical work on intensity-trapped solitons in the presence of group-velocity mismatch[17], such a

dual-state may not be able to exist on the pulse edge, and so in this example the left soliton is displaced by the right one and collapses. The remaining soliton continues to the edge of the pulse where it becomes locked[3].

The final high power DKS is depicted in Fig. S.5(e,f) in time and frequency respectively. Due to the Raman self-frequency shift, the dispersive-wave recoil of the spectrum center has been mostly canceled. Moreover, the increase in $\kappa_{\rm ex}$ at lower optical frequencies has caused the dispersive wave spectrum to broaden to 1.4 THz (3 dB width), agreeable with the experimental dispersive wave peak-width of 1.5 THz. Overall, a stable optical complex is formed comprising the background pulse, the Cherenkov radiation, and the soliton.

---

* tobias.kippenberg@epfl.ch


[1] T. Herr, V. Brasch, J. D. Jost, C. Y. Wang, N. M. Kondratiev, M. L. Gorodetsky, and T. J. Kippenberg, Nature Photonics **8**, 145 (2014).

[2] J. K. Jang, M. Erkintalo, S. Coen, and S. G. Murdoch, Nature Communications **6**, 7370 (2015).

[3] I. Hendry, W. Chen, Y. Wang, B. Garbin, J. Javaloyes, G.-L. Oppo, S. Coen, S. G. Murdoch, and M. Erkintalo, Physical Review A **97**, 10.1103/PhysRevA.97.053834 (2018).

[4] J. Liu, V. Brasch, M. H. P. Pfeiffer, A. Kordts, A. N. Kamel, H. Guo, M. Geiselmann, and T. J. Kippenberg, Optics Letters **41**, 3134 (2016).

[5] J. Liu, E. Lucas, A. S. Raja, J. He, J. Riemensberger, R. N. Wang, M. Karpov, H. Guo, R. Bouchand, and T. J. Kippenberg, arXiv:1901.10372 [physics] (2019), arXiv: 1901.10372.

[6] E. Obrzud, M. Rainer, A. Harutyunyan, B. Chazelas, M. Cecconi, A. Ghedina, E. Molinari, S. Kundermann, S. Lecomte, F. Pepe, F. Wildi, F. Bouchy, and T. Herr, Optics Express **26**, 34830 (2018).

[7] L. A. Lugiato and R. Lefever, Physical Review Letters **58**, 2209 (1987).

[8] S. Coen, H. G. Randle, T. Sylvestre, and M. Erkintalo, Optics Letters **38**, 37 (2013).

[9] M. Karpov, H. Guo, A. Kordts, V. Brasch, M. H. Pfeiffer, M. Zervas, M. Geiselmann, and T. J. Kippenberg, Physical Review Letters **116**, 103902 (2016).

[10] M. Haelterman, S. Trillo, and S. Wabnitz, Optics Communications **91**, 401 (1992).

[11] T. Herr, K. Hartinger, J. Riemensberger, C. Y. Wang, E. Gavartin, R. Holzwarth, M. L. Gorodetsky, and T. J. Kippenberg, Nature Photonics **6**, 480 (2012).

[12] F. Leo, L. Gelens, P. Emplit, M. Haelterman, and S. Coen, Optics Express **21**, 9180 (2013).

[13] C. Godey, I. V. Balakireva, A. Coillet, and Y. K. Chembo, Physical Review A **89**, 063814 (2014).

[14] S. Coulibaly, M. Taki, A. Bendahmane, G. Millot, B. Kibler, and M. G. Clerc, Physical Review X **9**, 011054 (2019).

[15] N. Akhmediev and M. Karlsson, Physical Review A **51**, 2602 (1995).

[16] C. Milin and D. V. Skryabin, Optics Express **22**, 3732 (2014).

[17] I. Hendry, B. Garbin, S. G. Murdoch, S. Coen, and M. Erkintalo, Physical Review A **100**, 023829 (2019).
